# Supplementary material for: Chemical Potentials and the One-Electron Hamiltonian of the Second-Order Perturbation Theory from the Functional Derivative Approach
Source: arXiv:2403.06405 ancillary file (2024-04-30)
Supplement: Supplementary file 1 [file supporting_information.pdf]

# Supporting Information: Chemical Potentials and the One-Electron Hamiltonian of the Second-Order Perturbation Theory from the Functional Derivative Approach

Jiachen Li[†,‡] and Weitao Yang[*,†]

†Department of Chemistry, Duke University, Durham, NC 27708, USA

‡Department of Chemistry, Yale University, New Haven, CT, USA 06520

E-mail: weitao.yang@duke.edu

## 1 MP2 derivative using the functional derivative approach

The derivative of the MP2 correlation energy with respect to the occupation number can be obtained from the functional derivative approach

$$\frac{dE_{\mathrm{c}}^{\mathrm{MP2}}}{dn_p} = \int_{-\infty}^{\infty} d\omega \frac{\delta E_{\mathrm{c}}^{\mathrm{MP2}}}{\delta G^0(\omega)} \frac{dG^0(\omega)}{dn_p} \tag{1}$$

where the functional derivative of the MP2 correlation energy to the non-interaction Green's function in Eq 1 is the second-order self-energy

$$\frac{\delta E_{\mathrm{c}}^{\mathrm{MP2}}}{\delta G_{pq}^0(\omega)} = \frac{1}{2\pi i} \Sigma_{pq}^{(2)}(\omega) \tag{2}$$

The fractional extension of the non-interaction Green's function $G^0$ in the real space is defined as[S1]

$$G^0(x_1,x_2,\omega)=\sum_i \frac{n_i\psi_i(x_1)\psi_i^*(x_2)}{\omega-\epsilon_i-i\eta}+\sum_a \frac{(1-n_a)\psi_a(x_1)\psi_a^*(x_2)}{\omega-\epsilon_a+i\eta} \tag{3}$$

Then the derivative of the non-interacting Green's function with respect to the occupation number consists of three parts

$$\begin{aligned}\frac{dG^0(x_1,x_2,\omega)}{dn_p} =&\frac{\partial G^0(x_1,x_2,\omega)}{\partial n_p}+\sum_q \frac{\partial G^0(x_1,x_2,\omega)}{\partial \epsilon_q}\frac{d\epsilon_q}{dn_p} \\ &+\sum_q\int dx_3\left[\frac{\delta G^0(x_1,x_2,\omega)}{\delta\psi_q(x_3)}\frac{d\psi_q(x_3)}{dn_p}+c.c\right]\end{aligned} \tag{4}$$

where

$$\frac{\partial G^0(x_1,x_2,\omega)}{\partial n_p} =\frac{-1}{\omega-\epsilon_p+i\eta}\psi_p(x_1)\psi_p^*(x_2)+\frac{1}{\omega-\epsilon_p-i\eta}\psi_p(x_1)\psi_p^*(x_2) \tag{5}$$

$$\frac{\partial G^0(x_1,x_2,\omega)}{\partial \epsilon_p} =\frac{1-n_p}{(\omega-\epsilon_p+i\eta)^2}\psi_p(x_1)\psi_p^*(x_2)+\frac{n_p}{(\omega-\epsilon_p-i\eta)^2}\psi_p(x_1)\psi_p^*(x_2) \tag{6}$$

$$\frac{\delta G^0(x_1,x_2,\omega)}{\delta \psi_p(x_3)} =\frac{1-n_p}{\omega-\epsilon_p+i\eta}\delta(x_1-x_3)\psi_p^*(x_2)+\frac{n_p}{\omega-\epsilon_p-i\eta}\delta(x_1-x_3)\psi_p^*(x_2) \tag{7}$$

Combining Eq.2 and Eq.4, the derivative of the MP2 correlation energy with respect to the occupation number is

$$\begin{aligned}\frac{dE_{\mathrm{c}}^{\mathrm{MP2}}}{dn_p} =&\int_{-\infty}^{\infty} d\omega \mathrm{Tr}\frac{\delta E_{\mathrm{c}}^{\mathrm{MP2}}}{\delta G_0(x_1,x_2,\omega)}\frac{dG_0(x_1,x_2,\omega)}{dn_p} \\ =&\frac{1}{2\pi i}\int_{-\infty}^{\infty} d\omega \mathrm{Tr}\Sigma^{(2)}(x_2,x_1,\omega)\left[\frac{\partial G_0(x_1,x_2,\omega)}{\partial n_p}+\sum_q\frac{\partial G_0(x_1,x_2,\omega)}{\partial\epsilon_q}\frac{d\epsilon_q}{dn_p}\right. \\ &\left.+\sum_q\int dx_3\left(\frac{\delta G_0(x_1,x_2,\omega)}{\delta\psi_q(x_3)}\frac{d\psi_q(x_3)}{dn_p}+c.c\right)\right] \\ =&\mathrm{I}+\mathrm{II}+\mathrm{III}\end{aligned} \tag{8}$$

Using Eq 5 we can get the first part of the MP2 derivative

$$
\begin{aligned}
\mathrm{I} =& \frac{1}{2\pi i}\int_{-\infty}^{\infty} d\omega \Sigma^{(2)}(x_2,x_1,\omega)\left[\frac{-1}{\omega-\epsilon_p+i\eta}\psi_p(x_1)\psi_p^*(x_2)+\frac{1}{\omega-\epsilon_p-i\eta}\psi_p(x_1)\psi_p^*(x_2)\right]\\
=& \frac{1}{2\pi i}\int_{-\infty}^{\infty} d\omega dx_1 dx_2 \Sigma^{(2)}(x_2,x_1,\omega)\left[\frac{-1}{\omega-\epsilon_p+i\eta}\psi_p(x_1)\psi_p^*(x_2)+\frac{1}{\omega-\epsilon_p-i\eta}\psi_p(x_1)\psi_p^*(x_2)\right]\\
=& \frac{1}{2\pi i}\int_{-\infty}^{\infty} d\omega \left[\Sigma_{pp}^{+(2)}(\omega)\frac{-1}{\omega-\epsilon_p+i\eta}+\Sigma_{pp}^{+(2)}(\omega)\frac{1}{\omega-\epsilon_p-i\eta}+\Sigma_{pp}^{-(2)}(\omega)\frac{-1}{\omega-\epsilon_p+i\eta}\right.\\
&\left.+\Sigma_{pp}^{-(2)}(\omega)\frac{1}{\omega-\epsilon_p-i\eta}\right]\\
=& \frac{1}{2\pi i}\int_{-\infty}^{\infty} d\omega \left[\Sigma_{pp}^{+(2)}(\omega)\frac{1}{\omega-\epsilon_p-i\eta}+\Sigma_{pp}^{-(2)}(\omega)\frac{-1}{\omega-\epsilon_p+i\eta}\right]\\
=& \Sigma_{pp}^{+(2)}(\epsilon_p)+\Sigma_{pp}^{-(2)}(\epsilon_p)\\
=& \Sigma_{pp}^{(2)}(\epsilon_p)
\end{aligned}
\tag{9}
$$

The integration in Eq.9 can be done on the complex plane with the residue theorem with the contour closing either on the upper or lower half plane. Only two terms after the third equals sign are non-zero because they have poles on both the upper and the lower plane. Using Eq 6 we can get the second part of the MP2 derivative

$$
\begin{aligned}
\mathrm{II} =& \frac{1}{2\pi i}\int_{-\infty}^{\infty} d\omega \mathrm{Tr}\Sigma^{(2)}(x_2,x_1,\omega)\sum_q \frac{\partial G_0(x_1,x_2,\omega)}{\partial \epsilon_q}\frac{d\epsilon_q}{dn_p}\\
=& \frac{1}{2\pi i}\int d\omega \mathrm{Tr}\Sigma^{(2)}(x_2,x_1,\omega)\sum_q\left[\frac{1-n_q}{(\omega-\epsilon_q+i\eta)^2}\psi_q(x_1)\psi_q^*(x_2)+\frac{n_q}{(\omega-\epsilon_q-i\eta)^2}\psi_q(x_1)\psi_q^*(x_2)\right]\frac{d\epsilon_q}{dn_p}\\
=& \frac{1}{2\pi i}\int_{-\infty}^{\infty} d\omega \sum_q\left[\Sigma_{qq}^{+(2)}(\omega)\frac{1-n_q}{(\omega-\epsilon_q+i\eta)^2}+\Sigma_{qq}^{+(2)}(\omega)\frac{n_q}{(\omega-\epsilon_q-i\eta)^2}\right.\\
&\left.+\Sigma_{qq}^{-(2)}(\omega)\frac{1-n_q}{(\omega-\epsilon_q+i\eta)^2}+\Sigma_{qq}^{-(2)}(\omega)\frac{n_q}{(\omega-\epsilon_q-i\eta)^2}\right]\frac{d\epsilon_q}{dn_p}\\
=& \frac{1}{2\pi i}\int_{-\infty}^{\infty} d\omega \sum_q\left[\Sigma_{qq}^{+(2)}(\omega)\frac{n_q}{(\omega-\epsilon_q-i\eta)^2}+\Sigma_{qq}^{-(2)}(\omega)\frac{1-n_q}{(\omega-\epsilon_q+i\eta)^2}\right]\frac{d\epsilon_q}{dn_p}\\
=& \sum_q\left[n_q\langle\psi_q|\frac{d\Sigma^{+(2)}(\omega)}{d\omega}\bigg|_{\omega=\epsilon_q}|\psi_q\rangle-(1-n_q)\langle\psi_q|\frac{d\Sigma^{-(2)}(\omega)}{d\omega}\bigg|_{\omega=\epsilon_q}|\psi_q\rangle\right]\frac{d\epsilon_q}{dn_p}
\end{aligned}
\tag{10}
$$

where $\frac{d\epsilon_q}{dn_p}$ is obtained from solving the CP-HF equation. Similar to Equation.9, only two terms after the third equals sign in Eq.10 are non-zero because they have poles on both the upper and the lower plane.

Using Eq 7 we can get the third part of the MP2 derivative

$$
\begin{aligned}
\text{III} =& \frac{1}{2\pi i}\int_{-\infty}^{\infty} d\omega \text{Tr}\Sigma^{(2)}(x_2,x_1,\omega)\sum_q\int dx_3\left[\frac{\delta G_0(x_1,x_2,\omega)}{\delta\psi_q(x_3)}\frac{d\psi_q(x_3)}{dn_p}+c.c\right] \\
=& \frac{1}{2\pi i}\sum_q\int_{-\infty}^{\infty} d\omega dx_1 dx_2 \Sigma^{(2)}(x_2,x_1,\omega)\left[\frac{1-n_q}{\omega-\epsilon_q+i\eta}\frac{d\psi_q(x_1)}{dn_p}\psi_q^*(x_2)\right. \\
& \left.+\frac{n_q}{\omega-\epsilon_q-i\eta}\frac{d\psi_q(x_1)}{dn_p}\psi_q^*(x_2)+c.c\right] \\
=& \sum_q\left[n_q\langle\psi_q|\Sigma^{+(2)}(\epsilon_q)|\frac{d\psi_q}{dn_p}\rangle-(1-n_q))\langle\psi_q|\Sigma^{-(2)}(\epsilon_q)|\frac{d\psi_q}{dn_p}\rangle\right. \\
& \left.+n_q\langle\frac{d\psi_q}{dn_p}|\Sigma^{+(2)}(\epsilon_q)|\psi_q\rangle-(1-n_q))\langle\frac{d\psi_q}{dn_p}|\Sigma^{-(2)}(\epsilon_q)|\psi_q\rangle\right] \\
=& \sum_q n_q\left[\langle\psi_q|\Sigma^{+(2)}(\epsilon_q)|\frac{d\psi_q}{dn_p}\rangle+\langle\frac{d\psi_q}{dn_p}|\Sigma^{+(2)}(\epsilon_q)|\psi_q\rangle\right] \\
& -\sum_q(1-n_q)\left[\langle\psi_q|\Sigma^{-(2)}(\epsilon_q)|\frac{d\psi_q}{dn_p}\rangle+\langle\frac{d\psi_q}{dn_p}|\Sigma^{-(2)}(\epsilon_q)|\psi_q\rangle\right]
\end{aligned}
\tag{11}
$$

where

$$
\langle\psi_q|\Sigma^{\pm(2)}(\epsilon_q)|\frac{d\psi_q}{dn_p}\rangle=\sum_r U_{rq}^p\langle\psi_q|\Sigma^{\pm(2)}(\epsilon_q)|\psi_r\rangle \tag{12}
$$

$$
\langle\frac{d\psi_q}{dn_p}|\Sigma^{\pm(2)}(\epsilon_q)|\psi_q\rangle=\sum_r U_{rq}^p\langle\psi_r|\Sigma^{\pm(2)}(\epsilon_q)|\psi_q\rangle \tag{13}
$$

with $U$ as the unitary matrix obtained from the CP-HF equation.

Combining all terms, we get a simple expression for the MP2 derivative

$$
\frac{dE_c^{\text{MP2}}}{dn_p}=\Sigma_{pp}^{+(2)}(\epsilon_p)+\Sigma_{pp}^{-(2)}(\epsilon_p)+\sum_q n_q\frac{d}{dn_p}\Sigma_{qq}^{+(2)}(\epsilon_q)-\sum_q(1-n_q)\frac{d}{dn_p}\Sigma_{qq}^{-(2)}(\epsilon_q) \tag{14}
$$

## 2 Equivalence of the functional derivative approach and the analytical approach for the MP2 derivative

In Ref. S2, the first term is related to the explicit dependence of the MP2 correlation energy on the occupation number

$$
\begin{aligned}
\frac{\partial E_c^{\mathrm{MP2}}}{\partial n_p} =& \frac{1}{2}\sum_{qrs}\frac{n_q(1-n_r)(1-n_s)\langle qt||rs\rangle^2}{\epsilon_q+\epsilon_p-\epsilon_r-\epsilon_s} - \frac{1}{2}\sum_{qrs}\frac{n_q n_r(1-n_s)\langle qr||ps\rangle^2}{\epsilon_q+\epsilon_r-\epsilon_p-\epsilon_s} \\
=& \Sigma_{pp}^{(2)}(\epsilon_p)
\end{aligned} \tag{15}
$$

which agrees with the first term in Eq.9.

The second term in Ref. S2 is related to the explicit dependence on the orbital energy.

$$
\begin{aligned}
\frac{\partial E_c^{\mathrm{MP2}}}{\partial \epsilon_p} =& - n_p\frac{1}{2}\sum_{qrs} n_q(1-n_r)(1-n_s)\frac{\langle pu||rs\rangle^2}{(\epsilon_q+\epsilon_u-\epsilon_r-\epsilon_s)^2} \\
&+ (1-n_p)\frac{1}{2}\sum_{qrs} n_q n_r(1-n_s)\frac{\langle qr||sp\rangle^2}{(\epsilon_q+\epsilon_r-\epsilon_s-\epsilon_p)^2} \\
=& n_p\frac{d\Sigma_{pp}^{(2)+}(\omega)}{d\omega}\bigg|_{\omega=\epsilon_p} - (1-n_p)\frac{d\Sigma_{pp}^{(2)-}(\omega)}{d\omega}\bigg|_{\omega=\epsilon_p}
\end{aligned} \tag{16}
$$

Then

$$
\sum_q \frac{\partial E_c^{\mathrm{MP2}}}{\partial \epsilon_q}\frac{d\epsilon_q}{dn_p} = \sum_q \left[ n_q\frac{d\Sigma_{qq}^{+(2)}(\omega)}{d\omega}\bigg|_{\omega=\epsilon_q} - (1-n_q)\frac{d\Sigma_{qq}^{-(2)}(\omega)}{d\omega}\bigg|_{\omega=\epsilon_q}\right]\frac{d\epsilon_q}{dn_p} \tag{17}
$$

which agrees with the the second term term in Eq.10.

The third term in Ref. S2 is related to the orbital relaxation effect.

$$
\begin{aligned}
\int dx_3 \frac{\delta E_c^{\mathrm{MP2}}}{\delta \phi_u(x_3)} \frac{d\psi_u(x_3)}{dn_t} =& \frac{1}{2} \sum_{prs} \frac{n_u n_p (1-n_r)(1-n_s)}{\epsilon_u + \epsilon_p - \epsilon_r - \epsilon_s} \langle \frac{du}{dn_t} p || rs \rangle \langle rs || up \rangle \\
&+ \frac{1}{2} \sum_{prs} \frac{n_u n_p (1-n_r)(1-n_s)}{\epsilon_u + \epsilon_p - \epsilon_r - \epsilon_s} \langle up || rs \rangle \langle rs || \frac{du}{dn_t} p \rangle \\
&- \frac{1}{2} \sum_{pqr} \frac{n_p n_q (1-n_r)(1-n_u)}{\epsilon_p + \epsilon_q - \epsilon_r - \epsilon_u} \langle pq || \frac{du}{dn_t} s \rangle \langle us || pq \rangle \\
&- \frac{1}{2} \sum_{pqr} \frac{n_p n_q (1-n_r)(1-n_u)}{\epsilon_p + \epsilon_q - \epsilon_r - \epsilon_u} \langle pq || us \rangle \langle \frac{du}{dn_t} s || pq \rangle \\
=& n_u \langle \psi_u | \Sigma^{+(2)}(\epsilon_u) | \frac{d\psi_u}{dn_t} \rangle + n_u \langle \frac{d\psi_u}{dn_t} | \Sigma^{+(2)}(\epsilon_u) | \psi_u \rangle \\
&- (1-n_u) \langle \psi_u | \Sigma^{-(2)}(\epsilon_u) | \frac{d\psi_u}{dn_t} \rangle - (1-n_u) \langle \frac{d\psi_u}{dn_t} | \Sigma^{-(2)}(\epsilon_u) | \psi_u \rangle
\end{aligned}
\tag{18}
$$

where we used the notation

$$
\frac{du}{dn_t} = \frac{d\psi_u}{dn_t} \tag{19}
$$

Therefore, this term agrees with the last term in our approach.

Adding all terms together, it can be seen that for the MP2 correlation energy, the derivative with respect to the occupation number from the approach in Ref. S2 is equivalent to our approach.

# 3 Derivation of the MP2 Hamiltonian

We first derive the equations for the variation of the non-interacting Green's function with respect to the density matrix. The density matrix is defined as

$$
\rho_s(x_1, x_2) = \sum_i \psi_i(x_1) \psi_i^*(x_2) = \sum_i \langle x_1 | \psi_i \rangle \langle \psi_i | x_2 \rangle \tag{20}
$$

and the density matrix for virtual states is given by

$$\bar{\rho}_s(x_1, x_2) = \sum_a \psi_a(x_1)\psi_a^*(x_2) = \sum_a \langle x_1|\psi_a\rangle\langle\psi_a|x_2\rangle \tag{21}$$

Therefore, the non-interacting Green's function can be written as

$$\begin{aligned} G^0(x_1, x_2, \omega) =& \sum_i \frac{n_i\psi_i(x_1)\psi_i^*(x_2)}{\omega - \epsilon_i - i\eta} + \sum_a \frac{(1-n_a)\psi_a(x_1)\psi_a^*(x_2)}{\omega - \epsilon_a + i\eta} \\ =& \sum_i \langle x_1|\frac{1}{\omega - \hat{h}_s - i\eta}|\psi_i\rangle\langle x_2|\psi_i\rangle + \sum_a \langle x_1|\frac{1}{\omega - \hat{h}_s + i\eta}|\psi_a\rangle\langle x_2|\psi_a\rangle \\ =& \langle x_1|\hat{g}(\omega - i\eta)\rho_s|x_2\rangle + \langle x_1|\hat{g}(\omega + i\eta)\bar{\rho}_s|x_2\rangle \end{aligned} \tag{22}$$

where $\hat{g}$ is defined as

$$\hat{g}(\omega) = \frac{1}{\omega - \hat{h}_s} \tag{23}$$

Thus, $G^0$ is a functional of $\rho_s$ because $\hat{h}_s$ is a functional of $\rho_s$, and we have the relation

$$I = \rho_s + \bar{\rho}_s \tag{24}$$

Using the operator identity

$$\frac{1}{A - B} = \frac{1}{A} + \frac{1}{A}B\frac{1}{A - B} \tag{25}$$

We have

$$\frac{1}{\omega - \hat{h}_s - \delta\hat{h}_s} = \frac{1}{\omega - \hat{h}_s} + \frac{1}{\omega - \hat{h}_s}\delta\hat{h}_s\frac{1}{\omega - \hat{h}_s - \delta\hat{h}_s} \tag{26}$$

To the first order of Eq.26

$$\frac{1}{\omega - \hat{h}_s - \delta\hat{h}_s} - \frac{1}{\omega - \hat{h}_s} = \frac{1}{\omega - \hat{h}_s}\delta\hat{h}_s\frac{1}{\omega - \hat{h}_s} \tag{27}$$

which means

$$\delta\hat{g}(\omega) = \hat{g}(\omega)\delta\hat{h}_s\hat{g}(\omega) \tag{28}$$

In Eq.28, the variation of the non-interacting Hamiltonian operator is

$$\delta\hat{h}_s(x_1,x_2) = \int dx_3 dx_4 f^{\mathrm{Hxc}}(x_1,x_2;x_4,x_3)\delta\rho_s(x_3,x_4) \tag{29}$$

or in short-hand notation

$$\delta\hat{h}_s = f^{\mathrm{Hxc}}\delta\rho_s \tag{30}$$

where $f^{\mathrm{Hxc}} = \frac{\delta\hat{h}_s}{\delta\rho_s}$ is the Hartree-exchange-correlation (Hxc) kernel. Thus, we can rewrite Eq.28 as

$$\delta\hat{g}(\omega) = \hat{g}(\omega)f^{\mathrm{Hxc}}\delta\rho_s\hat{g}(\omega) \tag{31}$$

Using Eq. 31 for the variation of $\hat{g}$ in Eq.22, we obtain the variation of the non-interacting Green's function

$$\begin{aligned}\delta G^0(\omega) =& \delta\hat{g}(\omega+i\eta)\bar{\rho}_s + \hat{g}(\omega+i\eta)\delta\bar{\rho}_s + \delta\hat{g}(\omega-i\eta)\rho_s + \hat{g}(\omega-i\eta)\delta\rho_s \\ =& \hat{g}(\omega+i\eta)f^{\mathrm{Hxc}}\delta\rho_s\hat{g}(\omega+i\eta)\bar{\rho}_s + \hat{g}(\omega-i\eta)f^{\mathrm{Hxc}}\delta\rho_s\hat{g}(\omega-i\eta)\rho_s \\ &+ [-\hat{g}(\omega+i\eta) + \hat{g}(\omega-i\eta)]\delta\rho_s\end{aligned} \tag{32}$$

Thus, the derivative of the non-interacting Green's function to the density matrix is

$$\begin{aligned}&\frac{\delta G(x_1,x_2,\omega)}{\delta\rho(x_3,x_4)} \\ =& g(x_1,x_5,\omega+i\eta)f^{\mathrm{Hxc}}(x_5,x_6,x_4,x_3)g(x_6,x_7,\omega+i\eta)\bar{\rho}_s(x_7,x_2) \\ &+ g(x_1,x_5,\omega-i\eta)f^{\mathrm{Hxc}}(x_5,x_6,x_4,x_3)g(x_6,x_7,\omega-i\eta)\rho_s(x_7,x_2) \\ &+ [-g(x_1,x_5,\omega+i\eta) + g(x_1,x_5,\omega-i\eta)]\delta(x_3,x_5)\delta(x_2,x_4)\end{aligned} \tag{33}$$

Note that for a complex $z$ with any finite imaginary part, the Eq.33 can be simplified as

$$\frac{\delta G(x_1,x_2,z)}{\delta\rho(x_3,x_4)} = g(x_1,x_5,z)f^{\mathrm{Hxc}}(x_5,x_6,x_4,x_3)g(x_6,x_7,z) \tag{34}$$

With the variation of the non-interacting Green's function in Eq.31, the variation of the

MP2 correlation energy is

$$
\begin{aligned}
&\delta E_{\mathrm{c}}^{\mathrm{MP2}}\\
=&\frac{1}{2\pi i}\int_{-\infty}^{\infty} d\omega \mathrm{Tr}[\Sigma_{st}^{(2)}(\omega)\delta G_{ts}^{0}(\omega)]\\
=&\frac{1}{2\pi i}\int_{-\infty}^{\infty} d\omega \mathrm{Tr}\frac{1}{2}\sum_{lmq}\langle sq||lm\rangle\langle lm||tq\rangle\Big\{\frac{(1-n_l)(1-n_m)n_q}{\omega-\epsilon_l-\epsilon_m+\epsilon_q+i\eta}+\frac{n_l n_m(1-n_q)}{\omega-\epsilon_l-\epsilon_m+\epsilon_q-i\eta}\Big\}\\
&\Big\{\Big(\hat{g}(\omega+i\eta)f^{\mathrm{Hxc}}\delta\rho_s\hat{g}(\omega+i\eta)\bar{\rho}_s\Big)_{ts}+\Big(\hat{g}(\omega-i\eta)f^{\mathrm{Hxc}}\delta\rho_s\hat{g}(\omega-i\eta)\rho_s\Big)_{ts}\\
&+\Big[\Big(-\hat{g}(\omega+i\eta)+\hat{g}(\omega-i\eta)\Big)\bar{\rho}_s\Big]_{ts}\Big\}\\
=&-\frac{1}{2}\mathrm{Tr}\sum_{lmq}\langle sq||lm\rangle\langle lm||tq\rangle(1-n_l)(1-n_m)n_q\Big(\hat{g}(\epsilon_l+\epsilon_m-\epsilon_q-i\eta)f^{\mathrm{Hxc}}\delta\rho_s\hat{g}(\epsilon_l+\epsilon_m-\epsilon_q-i\eta)\rho_s\Big)_{ts}\\
&+\frac{1}{2}\mathrm{Tr}\sum_{lmq}\langle sq||lm\rangle\langle lm||tq\rangle n_l n_m(1-n_q)\Big(\hat{g}(\epsilon_l+\epsilon_m-\epsilon_q+i\eta)f^{\mathrm{Hxc}}\delta\rho_s\hat{g}(\epsilon_l+\epsilon_m-\epsilon_q+i\eta)\bar{\rho}_s\Big)_{ts}\\
&+\frac{1}{2\pi i}\int_{-\infty}^{\infty} d\omega\Sigma^{(2)}(x_2,x_1,\omega)\int dx_3\{\sum_t 2\pi\delta(\omega-\epsilon_t)\psi_t(x_1)\psi_t^*(x_3)\delta\rho_s(x_3,x_2)\}
\end{aligned}
\tag{35}
$$

$$
\begin{aligned}
=&-\frac{1}{2}\mathrm{Tr}\sum_{lmquv}\langle sq||lm\rangle\langle lm||tq\rangle(1-n_l)(1-n_m)n_q \\
&\left(\hat{g}(\epsilon_l+\epsilon_m-\epsilon_q-i\eta)\right)_{tu}\left(f^{\mathrm{Hxc}}\delta\rho_s\right)_{uv}\left(\hat{g}(\epsilon_l+\epsilon_m-\epsilon_q-i\eta)\right)_{vs}n_s \\
&+\frac{1}{2}\mathrm{Tr}\sum_{lmquv}\langle sq||lm\rangle\langle lm||tq\rangle n_l n_m(1-n_q) \\
&\left(\hat{g}(\epsilon_l+\epsilon_m-\epsilon_q+i\eta)\right)_{tu}\left(f^{\mathrm{Hxc}}\delta\rho_s\right)_{uv}\left(\hat{g}(\epsilon_l+\epsilon_m-\epsilon_q+i\eta)\right)_{vs}(1-n_s) \\
&+\mathrm{Tr}\sum_{t}\Sigma^{(2)}(\epsilon_t)|\psi_t\rangle\langle\psi_t|\delta\rho_s \\
=&-\frac{1}{2}\mathrm{Tr}\sum_{lmquv}\langle sq||lm\rangle\langle lm||tq\rangle(1-n_l)(1-n_m)n_q \\
&\delta_{tu}\frac{1}{\epsilon_l+\epsilon_m-\epsilon_q-\epsilon_t-i\eta}\left(f^{\mathrm{Hxc}}\delta\rho_s\right)_{uv}\delta_{vs}\frac{1}{\epsilon_l+\epsilon_m-\epsilon_q-\epsilon_s-i\eta}n_s \\
&+\frac{1}{2}\mathrm{Tr}\sum_{lmquv}\langle sq||lm\rangle\langle lm||tq\rangle n_l n_m(1-n_q) \\
&\delta_{tu}\frac{1}{\epsilon_l+\epsilon_m-\epsilon_q-\epsilon_t+i\eta}\left(f^{\mathrm{Hxc}}\delta\rho_s\right)_{uv}\delta_{vs}\frac{1}{\epsilon_l+\epsilon_m-\epsilon_q-\epsilon_s+i\eta}(1-n_s) \\
&+\mathrm{Tr}\sum_{t}\Sigma^{(2)}(\epsilon_t)|\psi_t\rangle\langle\psi_t|\delta\rho_s \\
=&-\frac{1}{2}\sum_{lmqst}\langle sq||lm\rangle\langle lm||tq\rangle(1-n_l)(1-n_m)n_q n_s\frac{1}{\epsilon_l+\epsilon_m-\epsilon_q-\epsilon_t}\frac{1}{\epsilon_l+\epsilon_m-\epsilon_q-\epsilon_s}\left(f^{\mathrm{Hxc}}\delta\rho_s\right)_{ts} \\
&+\frac{1}{2}\sum_{lmqst}\langle sq||lm\rangle\langle lm||tq\rangle n_l n_m(1-n_q)(1-n_s)\frac{1}{\epsilon_l+\epsilon_m-\epsilon_q-\epsilon_t}\frac{1}{\epsilon_l+\epsilon_m-\epsilon_q-\epsilon_s}\left(f^{\mathrm{Hxc}}\delta\rho_s\right)_{ts} \\
&+\frac{1}{2}\sum_{st}\left\{\langle s|\Sigma^{(2)}(\epsilon_t)|t\rangle\langle t|\delta\rho_s|s\rangle+c.c(\epsilon_t\to\epsilon_s)\right\}
\end{aligned}
\tag{36}
$$

Therefore, the correlation part of the MP2 Hamiltonian is

$$
\begin{aligned}
&[H_{\mathrm{c}}^{\mathrm{MP2}}]_{st} \\
=&\frac{\delta E_{\mathrm{c}}^{\mathrm{MP2}}}{\delta(\rho_s)_{st}} \\
=&-\frac{1}{2}\sum_{lmquv}\langle uq||lm\rangle\langle lm||vq\rangle(1-n_l)(1-n_m)n_q n_u\frac{1}{\epsilon_l+\epsilon_m-\epsilon_q-\epsilon_u}\frac{1}{\epsilon_l+\epsilon_m-\epsilon_q-\epsilon_v}f^{\mathrm{Hxc}}_{uv,ts} \\
&+\frac{1}{2}\sum_{lmquv}\langle uq||lm\rangle\langle lm||vq\rangle n_l n_m(1-n_q)(1-n_u)\frac{1}{\epsilon_l+\epsilon_m-\epsilon_q-\epsilon_u}\frac{1}{\epsilon_l+\epsilon_m-\epsilon_q-\epsilon_v}f^{\mathrm{Hxc}}_{us,ts} \\
&+\frac{1}{2}\left\{\langle s|\Sigma^{(2)}(\epsilon_t)|t\rangle+\langle t|\Sigma^{(2)}(\epsilon_s)|s\rangle\right\} \\
=&-\frac{1}{2}\sum_{ijabp}\langle ij||ab\rangle\langle ab||pi\rangle\frac{1}{\epsilon_a+\epsilon_b-\epsilon_i-\epsilon_p}\frac{1}{\epsilon_a+\epsilon_b-\epsilon_i-\epsilon_j}f^{\mathrm{Hxc}}_{pj,ts} \\
&+\frac{1}{2}\sum_{ijabp}\langle ba||ij\rangle\langle ij||pa\rangle\frac{1}{\epsilon_i+\epsilon_j-\epsilon_a-\epsilon_p}\frac{1}{\epsilon_i+\epsilon_j-\epsilon_a-\epsilon_b}f^{\mathrm{Hxc}}_{pb,ts} \\
&+\frac{1}{2}\left\{\langle s|\Sigma^{(2)}(\epsilon_t)|t\rangle+\langle t|\Sigma^{(2)}(\epsilon_s)|s\rangle\right\}
\end{aligned}
\tag{37}
$$

where we have used

$$\left(f^{\mathrm{Hxc}}\delta\rho_s\right)_{pq}=\sum_{rs}f^{\mathrm{Hxc}}_{pq,rs}[\delta\rho_s]_{sr} \tag{38}$$

# References


(S1) Yang, W.; Mori-Sánchez, P.; Cohen, A. J. Extension of Many-Body Theory and Approximate Density Functionals to Fractional Charges and Fractional Spins. *J. Chem. Phys.* **2013**, *139*, 104114.

(S2) Su, N. Q.; Xu, X. Integration Approach at the Second-Order Perturbation Theory: Applications to Ionization Potential and Electron Affinity Calculations. *J. Chem. Theory Comput.* **2015**, *11*, 4677–4688.
